# Supplementary material for: Staging superstructures in high-$T_c$ Sr/O co-doped La$_{2-x}$Sr$_x$CuO$_{4+y}$
Source: arXiv:1707.08871 ancillary file (2017-08-11)
Supplement: Supplementary file 1 [file supplementary.pdf]

# SUPPLEMENTARY MATERIAL TO:

## Staging superstructures in high-$T_c$ Sr/O co-doped $La_{2-x}Sr_xCuO_{4+y}$

P. J. Ray,[1,*] N. H. Andersen,[2] T. B. S. Jensen,[2] H. E. Mohottala,[3,4] Ch. Niedermayer,[5] K. Lefmann,[1] B. O. Wells,[3] M. v. Zimmermann,[6] and L. Udby[1]

[1] *Nanoscience Center, Niels Bohr Institute, University of Copenhagen, DK-2100 Copenhagen, Denmark*
[2] *Physics Department, Technical University of Denmark, DK-2800 Kgs. Lyngby, Denmark*
[3] *Department of Physics, University of Connecticut U-3046, 2152 Hillside Road, Storrs, Connecticut 06269-3046, USA*
[4] *Department of Physics, University of Hartford, 200, Bloomfield Ave., West Hartford, CT-06117, USA*
[5] *Laboratory for Neutron Scattering, ETHZ & PSI, Ch-5232 Villigen PSI, Switzerland*
[6] *Deutsches Elektronen-Synchrotron DESY, Notkestr. 85, 22603 Hamburg, Germany*

(Dated: August 11, 2017)

### ESTIMATE OF OXYGEN CONTENTS

It is possible to give an estimate of the oxygen doping content ($y$) in the samples by assuming that the entire sample is either superconducting with $n_h = 0.16$ or magnetic with $n_h = 0.125$. Knowing the magnetic or superconducting volume fractions, $V_{\rm m}$ and $V_{\rm SC} = 1 - V_{\rm m}$ respectively (from separate measurements which agree with this relation), the value of $y$ can then be determined as

$$y_{\rm simple} = \frac{0.125V_{\rm m} + 0.16V_{\rm SC} - x}{2},$$

where $x$ is the Sr doping. This estimate comes from the standard assumption that each doped Sr supplies one electron to the $CuO_6$ planes, while each doped O supplies 2 such that the total hole doping is $n_h = x+2y = 0.125V_{\rm m}+0.16V_{\rm SC}$. It has, however, also been argued that for total hole dopings $n_h > 0.06$ the doping efficiency of the added oxygen is only 1.3 holes per O, [1].

Using this alternative relation, it is possible to get a slightly different estimate of the oxygen doping value $y = y_1+y_2$ from $n_h = x+2y_1+1.3y_2$. Here, $x+2y_1 \leq 0.06$ gives the value of $y_1$ as $(0.06-x)/0.5$ for dopings where $x$ does not exceed 0.06 on it's own (if it does, $y_1$ is simply 0). With that, it is simple to see that $y_2 = (n_h-x-2y_1)/1.3 = (n_h-0.06)/1.3$, and hence

$$y_{\rm advanced} = \begin{cases} \dfrac{0.06-x}{2} + \dfrac{0.125V_{\rm m} + 0.16V_{\rm SC} - 0.06}{1.3} & \text{for } x \leq 0.06, \\ \dfrac{0.125V_{\rm m} + 0.16V_{\rm SC} - x}{1.3} & \text{for } x > 0.06. \end{cases}$$

Using values from Ref. [2] for the $x = 0.04$, 0.065, and 0.09 samples, and results from not yet published data on the $x = 0.00$ sample, this results in the following values for $y$:

| $x$ | $V_{\rm m}$ | $V_{\rm SC}$ | $V_{\rm SC}/V_{\rm m}$ | $y_{\rm simple}$ | $y_{\rm advanced}$ |
|---|---|---|---|---|---|
| 0.00 | 0.66(5) | 0.37(5) | 0.56 | 0.071(7) | 0.093(7) |
| 0.04 | 0.56(1) | 0.44(1) | 0.79 | 0.050(4) | 0.072(4) |
| 0.065 | 0.19(1) | 0.81(1) | 4.26 | 0.044(2) | 0.068(2) |
| 0.09 | 0.53(1) | 0.47(1) | 1.13 | 0.027(1) | 0.041(1) |

An actual measurement of the oxygen content in the samples would require destructive methods, such as the TGA measurements mentioned briefly in Ref. [3] for the $x = 0.065$ sample. These measurements yielded $y = 0.032(5)$. However, subsequent measurements done on the other samples yielded very inconsistent results.

## PEAK POSITIONS AND WIDTHS FOR THE $x = 0.04$ SAMPLE FITS

The (014) peak $l$-scans for the $x = 0.04$ sample was fit to three Lorentzians at each temperature, with integrated intensities as shown in Fig. 3 in the main paper. The positions of these peaks (including the center between the position of the two staging peaks), as well as the widths of the staging peaks, are shown in Fig. 1.

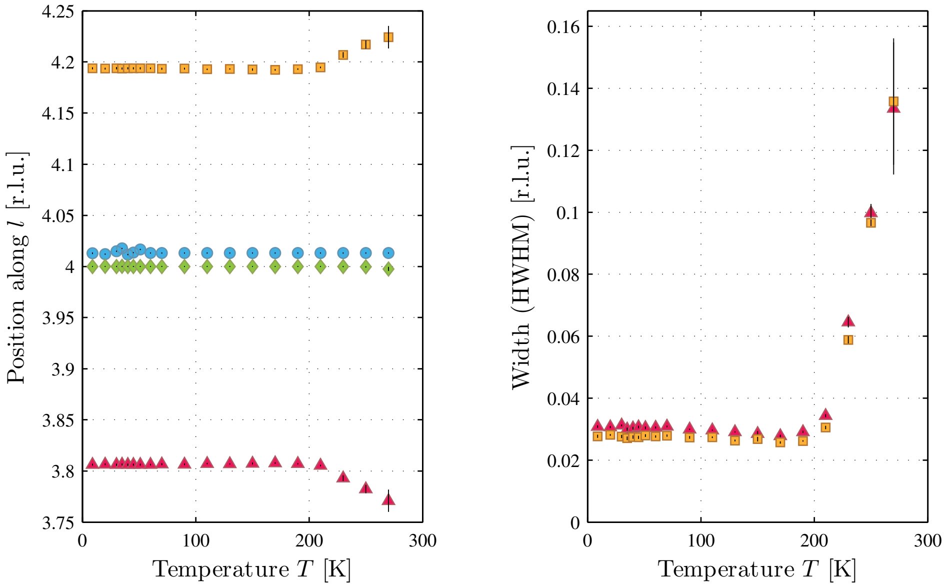


FIG. 1: Overview of peak positions (left) and staging peak widths (right) for the $x = 0.04$ sample. Blue points show the position of the central *Bmab* peak while green diamonds show the mid-point of the staging peaks, which are in turn positioned at the yellow squares and red triangles.

There is a clear difference between the blue points and the green diamonds in the figure, indicating different $c$ axis lengths for the *Bmab* and the staged structures. Note that the *Bmab* peak position was held fixed in the fit to the $T = 60$ K value above this temperature.

The widths of the staging peaks show a clear increase around the phase transition, as expected for a second order phase transition.

## GRADIENT ANALYSIS AS AN ALTERNATIVE METHOD TO FIND THE CRITICAL TEMPERATURE

For some of the samples, the data was very sparse near the transition, and an alternative method than fitting directly with a power law was needed to find the transition temperature. We define the transition temperature as the temperature where the slope of the data curve is the highest, along the lines of Ref. [4]. In order to do this analysis the integrated intensity data has been interpolated linearly and smoothed with a low-pass Butterworth filter in order to find the gradient in a meaningful way. This is illustrated in Fig. 2.

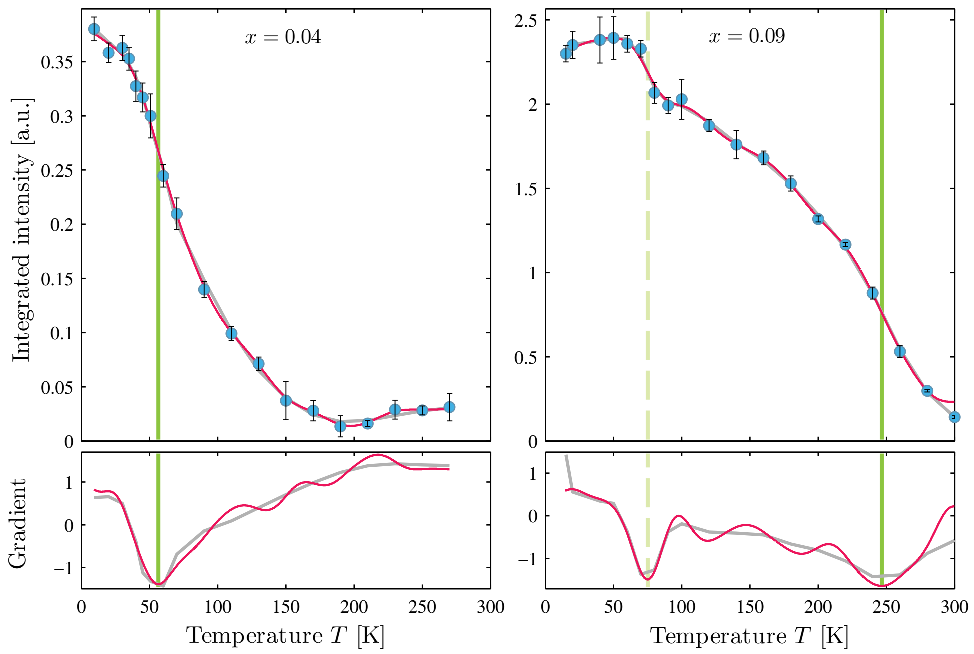


FIG. 2: Gradient analysis of the central *Bmab* peaks for the $x = 0.04$ and 0.09 samples, where an alternative analysis was needed in order to locate the transition temperature for the power law fits shown in Fig. 3 in the main paper (following Ref. [4]). The data is smoothened with a low-pass Butterworth filter, resulting in the red lines in the top plots, of which the gradient is then taken, shown as red lines in the bottom plots. The simple gradient directly between the datapoints is shown underneath in gray. The minimum of the gradient indicates the transition temperature of the phase transition. Note how the second minimum (dashed green line) could indicate a second lower temperature phase transition for the $x = 0.09$ sample.

This method gave results in agreement with the results found directly through fitting in the datasets where this was possible. Power law fits using this method to fix a transition temperature (for the $x = 0.00$ sample) and with free transition temperature as a fitting parameter (for the $x = 0.065$ and 0.09 samples), are shown for the staging signals with dashed lines in Fig. 3 in the main paper.

## POSSIBILITY FOR SEVERAL STAGING PEAKS OVERLAPPING FOR THE $x = 0.00$ SAMPLE

It is interesting to look at the main staging peaks for the $x = 0.00$ sample at a variety of temperatures (in Fig. 3 is shown $T = 10$, 161, and 220 K). It is visible how the peaks narrow at higher temperature, and seemingly move towards the center position. The peak likely consist of signals from several different staging domains of slightly different staging number, with the higher staging number domain gradually disappearing as temperature is increased.

Through the data analysis, the central peak has been fitted as a single peak – limited by the fact that many other separate peaks are also fitted, resulting in too many fitting parameters in the case of adding extra peaks. This results in the integrated intensity overview in the paper seemingly having several phase transitions. These peaks could also be treated as two separate, but overlapping, peaks, and fitted individually – hopefully resulting in two visibly different transition temperatures. This was, unfortunately, not practical due to the already large number of fitting parameters used to fit the peak data. Further measurements close to both of the transitions could be very interesting.

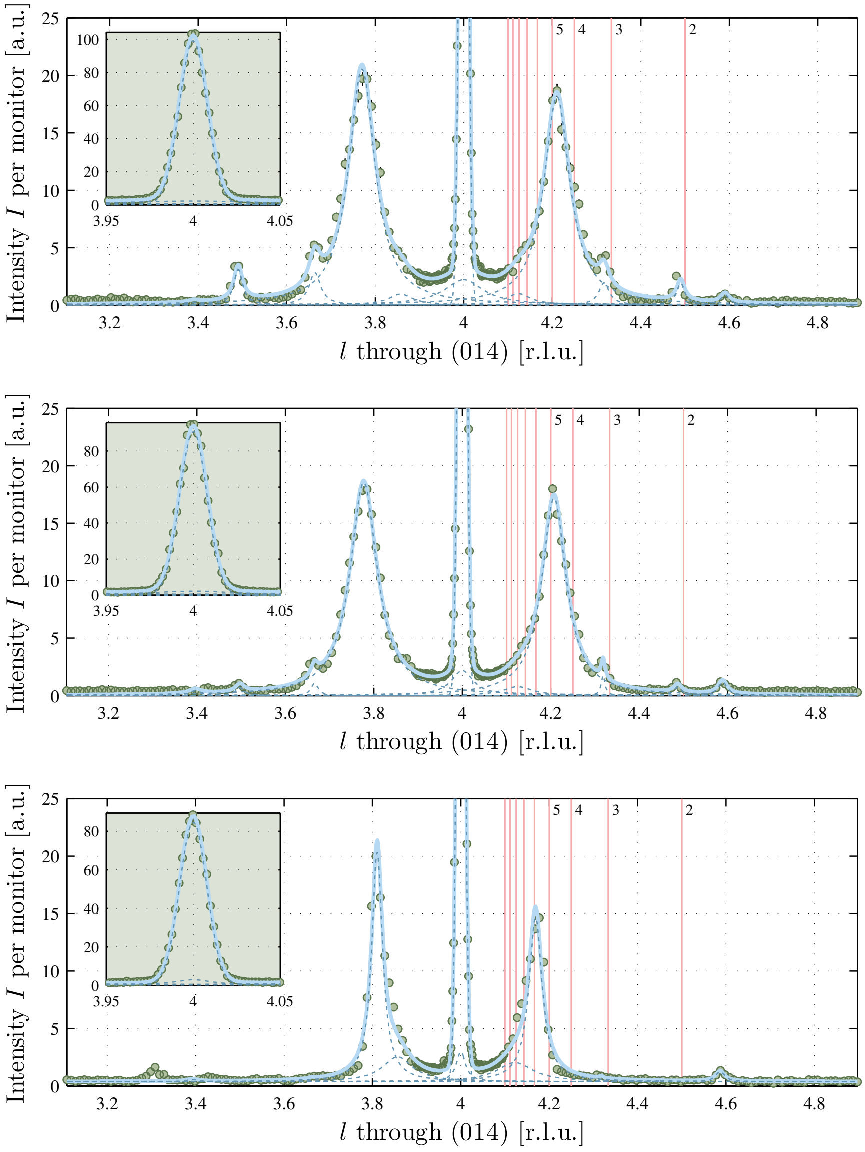


FIG. 3: Examples of fits done for the $x = 0.00$ sample, here for the (top) $T = 10\,\text{K}$, (middle) $T = 161\,\text{K}$, and (bottom) $T = 220\,\text{K}$ measurements. The individual peaks of the fit are shown as dashed lines (plus the constant background), while the full fit is the solid blue line. The vertical orange lines in the background mark integer staging positions on the high $l$ side up to $n = 10$, with $n$ indicated in the top for the smaller values. For points without visible errorbars, the errors are smaller than the marker. The insets show zoom-ins of the central peak in its full height.

## OVERVIEW OF TRANSITION TEMPERATURE RESULTS

The found transition temperatures for both staging and central *Bmab* peaks are shown in Fig. 4, compared to the transition temperature for the *Bmab* signal for the oxygen-stoichiometric compound, which is well known [5] (shown in green).

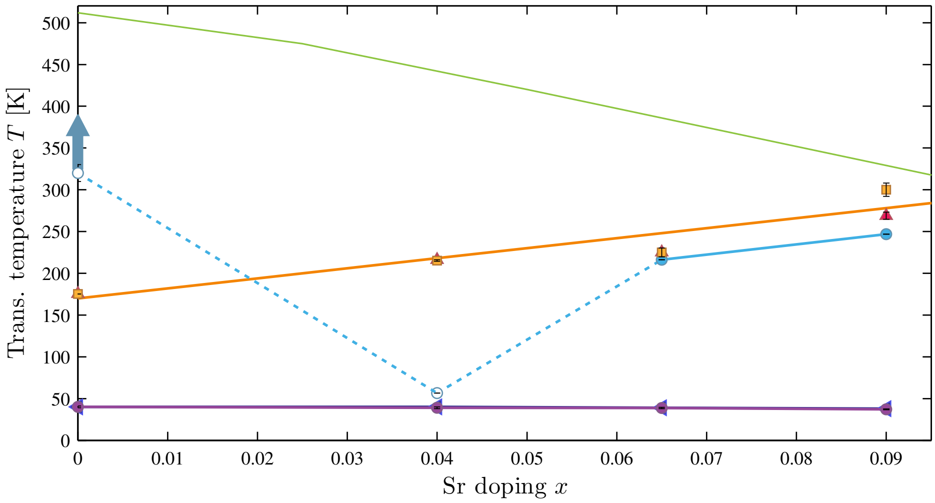


FIG. 4: Transition temperature obtained with the direct power law fits of low temperature data as well as using the slope method as explained elsewhere in this supplementary document. Shown points are for staging (red triangles for low $l$ and yellow squares for high $l$) and central (blue circles) peaks, with the well known tetragonal to ortorhombic transition for oxygen stoichiometric $La_{2-x}Sr_xCuO_4$ (green thin line) [5, 6]. Earlier found $T_N$ and $T_c$ for each sample are marked in blue triangles and purple circles (overlapping) [2]. The transition temperature for the central peak observed for the $x = 0.00$ sample has been found elsewhere to be above the maximum of 300 K used in the present experiments [7] (indicated with an arrow on the point). The central peak results for the $x = 0.04$ sample are marked by empty circles, noting the uncertainties of the phase transition temperature because of the width of the transition. The straight orange line is a guide to the eye for the staging transition temperatures.

## ABOUT THE HIGH STAGING NUMBERS AND PEAK WIDTHS

Typical widths of low-temperature staging peaks along $l$ for the $x = 0.09$ sample are HWHM = 0.0022 Å$^{-1}$, corresponding to typical correlation lengths in the order of $\pi$/HWHM = 1400 Å (assuming experimental resolution is negligible), or about 110 unit cells along $c$. This is indeed a larger correlation length than the $n/2 = 44.5$ unit cells needed for inferring a staging number of 90 for the sample.

## (004) AND (014) SCANS AT LOW TEMPERATURE FOR $x = 0.065$ SAMPLE

In order to account for the hints of staging in the sample rotation scan on the $x = 0.065$ sample presented in the main text, we also performed $(\theta, 2\theta)$ scans for the (004) and (014) peaks at low temperature, where the staging is assumed to be fully developed. These are shown in Fig. 5.

We can then compare the peak shape, and see that the (014) peak indeed shows a broadening that could be interpreted as staging, as shown in Fig. 6.

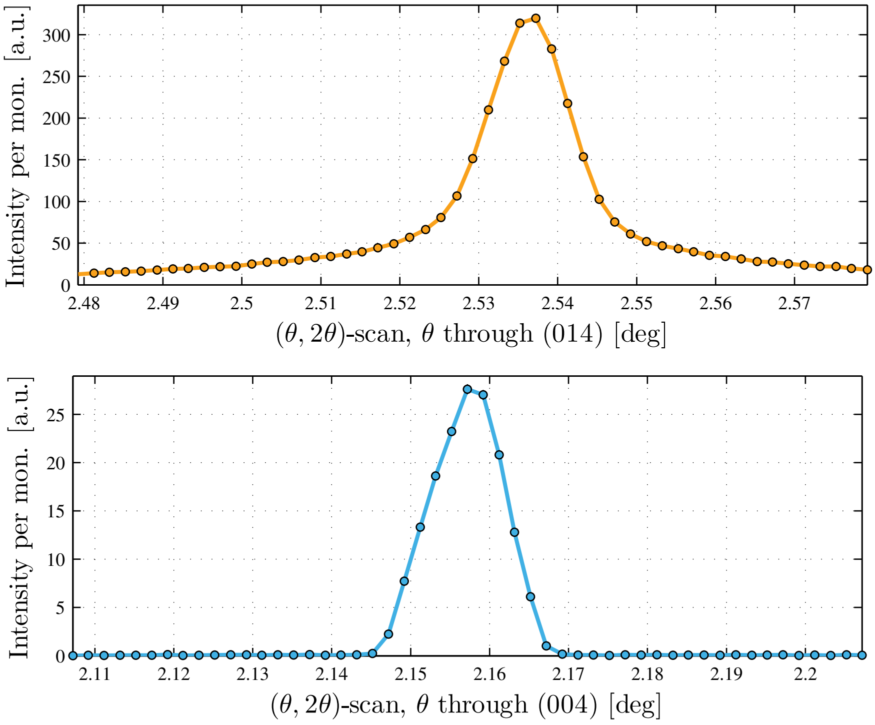


FIG. 5: Scans of (top) the (014) and (bottom) the (004) peaks, to compare the peak shape – as combined in Fig. 6. These are both at what is considered low temperature, at 6 K and 67 K, for the (014) and (004) peak, respectively.

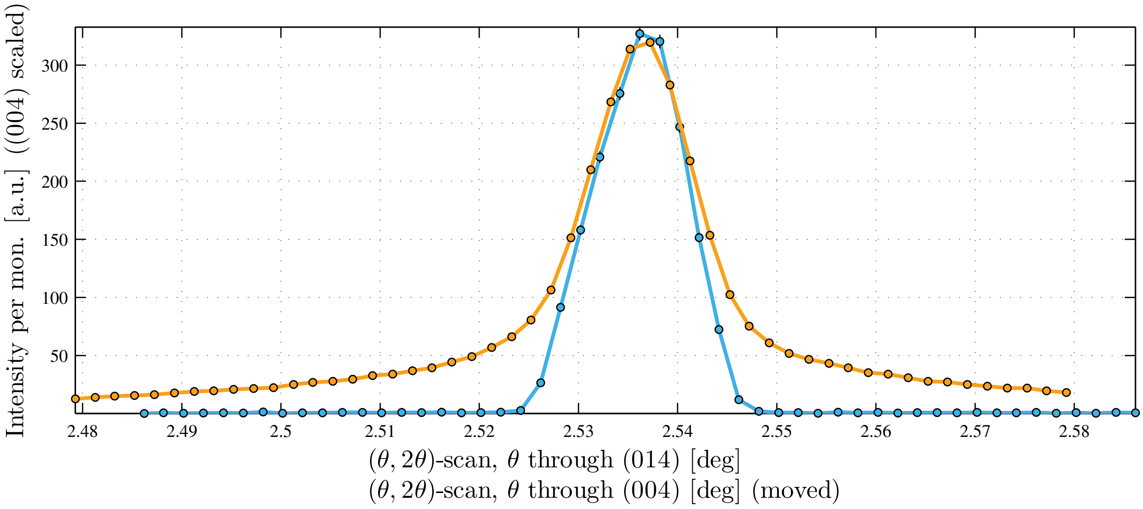


FIG. 6: The peaks in Fig. 5 overlapped, with the (004) peak (at $T = 67$ K) scaled and moved to have same center and maximum intensity as the (014) peak (at $T = 6$ K), for easy comparison.

## (014) SCANS AT HIGH AND LOW TEMPERATURE FOR $x = 0.09$ SAMPLE

In order to account for hints of staging in the $x = 0.09$ sample, we compare the room temperature and low temperature measurements along $l$. Scaling the room temperature data to the low temperature data, as shown in Fig. 7, it is clearly seen how the low temperature data is wider. Note also the spurious shoulder on the high $l$ side of the room temperature peak.

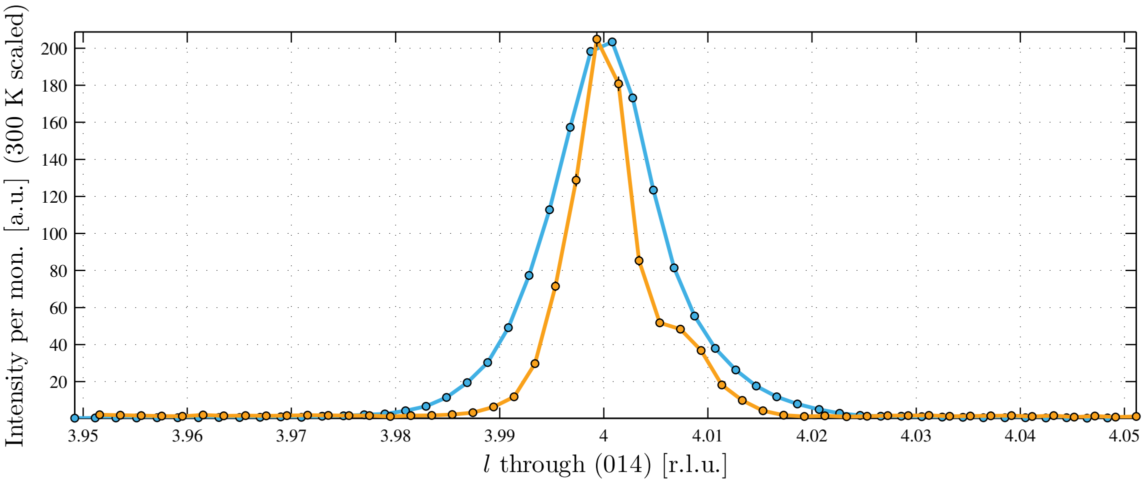


FIG. 7: The (014) peak at $T = 15$ K (blue points) and $T = 300$ K (yellow points), with he room temperature data scaled down to the same maximum intensity as the low-temperature data, in order to compare the peak shape.

## DISCUSSION REGARDING INSTRUMENT RESOLUTION

With regards to the (004) transverse and longitudinal widths not being directly comparable to the widths seen in the $[0KL]$ grid scans: Unfortunately, the sample was not measured with $[0KL]$ in the horizontal plane. The reason for the spread in $\omega$ widths between the different locations in the grid shown in Fig. 1(d) in the main text, is that the scans were not performed in-plane ($\chi$ scan) due to the mounting of the crystals.

* Corresponding author: pia@pjray.dk


[1] Z. G. Li, H. H. Feng, Z. Y. Yang, A. Hamed, S. T. Ting, and P. H. Hor, Physical Review Letters **77**, 5413 (1996).

[2] L. Udby, J. Larsen, N. B. Christensen, M. Boehm, C. Niedermayer, H. E. Mohottala, T. B. S. Jensen, R. Toft-Petersen, F. C. Chou, N. H. Andersen, et al., Physical Review Letters **111**, 227001 (2013), ISSN 0031-9007.

[3] H. E. Mohottala, B. O. Wells, J. I. Budnick, W. A. Hines, C. Niedermayer, L. Udby, C. Bernhard, A. R. Moodenbaugh, and F.-C. Chou, Nature Materials **5**, 377 (2006), ISSN 1476-1122.

[4] A. D. Bruce, Journal of Physics C **14**, 193 (1981).

[5] S. Wakimoto, H. Kimura, M. Fujita, K. Yamada, Y. Noda, G. Shirane, G. Gu, H. Kim, and R. J. Birgeneau, Journal of the Physical Society of Japan **75**, 074714 (2006), ISSN 0031-9015.

[6] J. Chang, Dissertation (phd thesis), Eidg. Technische Hochschule Zürich (2008).

[7] P. Radaelli, J. Jorgensen, R. Kleb, B. Hunter, F. Chou, and D. Johnston, Physical Review B **49**, 6239 (1994).
